# Supplementary material for: Nonequilibrium quasistationary spin disordered state in the Kitaev-Heisenberg magnet $\alpha$-RuCl$_3$
Source: arXiv:2005.14189 ancillary file (2020-05-28)
Supplement: Supplementary file 1 [file supplmatRuCl3noneq.pdf]

# Supplementary Materials for “Nonequilibrium quasistationary spin disordered state in the Kitaev-Heisenberg magnet $\alpha$ -RuCl<sub>3</sub>”

R. B. Versteeg,<sup>1,\*,\dagger</sup> A. Chiocchetta,<sup>2</sup> F. Sekiguchi,<sup>1</sup> A. I. R. Aldea,<sup>1</sup>  
A. Sahasrabudhe,<sup>1</sup> K. Budzinauskas,<sup>1</sup> Zhe Wang,<sup>1</sup> V. Tsurkan,<sup>3,4</sup>  
A. Loidl,<sup>3</sup> D. I. Khomskii,<sup>1</sup> S. Diehl,<sup>2</sup> P. H. M. van Loosdrecht<sup>1,\*\*</sup>

<sup>1</sup> Institute of Physics II, University of Cologne, D-50937 Cologne, Germany

<sup>2</sup> Institute for Theoretical Physics, University of Cologne, D-50937 Cologne, Germany

<sup>3</sup> Experimental Physics V, Center for Electronic Correlations and Magnetism,  
University of Augsburg, 86159 Augsburg, Germany

<sup>4</sup> Institute of Applied Physics, MD 2028, Chisinau, Republic of Moldova

\* Corresponding author: rolf.versteeg@epfl.ch

<sup>\dagger</sup> Current address: Laboratoire de Spectroscopie Ultrarapide  
and Lausanne Centre for Ultrafast Science (LACUS), ISIC-FSB,  
École Polytechnique Fédérale de Lausanne, CH-1015 Lausanne, Switzerland

\*\* Corresponding author: pvl@ph2.uni-koeln.de

# S1 Photoexcited holon-doublon pair density

## S1.1 Optical penetration depth

The optical conductivity  $\sigma_1(\omega)$  is obtained from Ref.1, and shown in Fig. S1a. Kramers-Kronig analysis is performed to obtain  $\sigma_2(\omega)$ . The result is shown in Fig. S1a. From  $\sigma(\omega) = \sigma_1(\omega) + i\sigma_2(\omega)$  the relative dielectric permittivity is obtained by:

$$\epsilon_r(\omega) = \epsilon_1(\omega) + i\epsilon_2(\omega) = 1 + \frac{1}{4\pi\epsilon_0} \frac{i\sigma(\omega)}{\omega} \quad (\text{S1})$$

From  $\epsilon_r(\omega)$  one obtains the refractive index  $\tilde{n} = n(\omega) + i\kappa(\omega)$ , to finally calculate the absorption coefficient  $\alpha(\omega)$  by:

$$\alpha(\omega) = \frac{4\pi\kappa(\omega)}{\lambda} \quad (\text{S2})$$

with  $\lambda$  the wavelength. The absorption coefficient (shown in Fig. S1b) is calculated into the optical penetration depth by  $\delta(\omega) = 1/\alpha(\omega)$ . For the pump photons a penetration depth  $\delta(1.55\text{eV}) \approx 0.65\mu\text{m}$  is calculated, and for the probe photons  $\delta(1.55\text{eV}) \approx 0.23\mu\text{m}$ , as also indicated in Fig. S1c. Finally, the reflection coefficient is calculated (not shown).

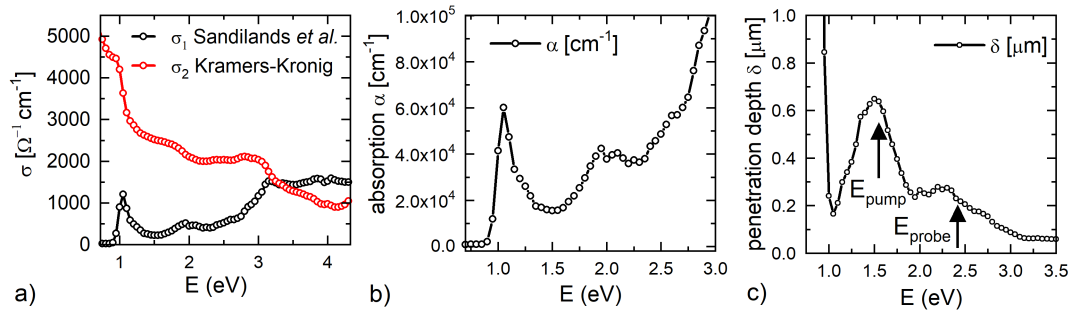

**Figure S1:** a) The real part of the optical conductivity  $\sigma_1$  is obtained from Ref.1. The imaginary part  $\sigma_2$  is obtained by Kramers-Kronig analysis. b) The absorption coefficient  $\alpha$ . c) The corresponding optical penetration depth  $\delta$ . The pump and probe photon energies are indicated with arrows.

## S1.2 Photoexcitation density

Table S1 summarizes crystallographic properties needed to calculate the photoexcited holon-doublon density.

**Table S1:** Properties of  $\alpha$ -RuCl<sub>3</sub>

| property                                | value                    |          |
|-----------------------------------------|--------------------------|----------|
| unit cell volume $V_{\text{u.c.}}$      | 371 Å <sup>3</sup>       | (Ref. 2) |
| chemical unit formulas in unit cell $Z$ | 4                        | (Ref. 2) |
| molar mass $m$                          | 207.43 amu               |          |
| density $\rho$                          | 3.7123 g/cm <sup>3</sup> |          |

Given the pump penetration depth  $\delta_{\text{pump}}(1.55\text{eV})$  and spot radius  $r_{\text{pump}} \approx 39 \mu\text{m}$ , we obtain a  $V_{\text{pump}} \approx 3.06 \cdot 10^{-9} \text{ cm}^3$ . This means there are:

$$N_{\text{Ru}} = \frac{Z \cdot V_{\text{pump}}}{V_{\text{u.c.}}} \approx 3.3 \cdot 10^{13} \quad (\text{S3})$$

Ru-ions in the pump volume. For a pump power  $P = 1 \mu\text{W}$  at a repetition rate  $f = 30 \text{ kHz}$ , the pulse energy is given by  $E_{\text{pulse}} \approx 0.033 \text{ nJ}$ , corresponding to a fluence  $F \approx 0.7 \mu\text{J}/\text{cm}^2$ . With pump photon energy  $1.55 \text{ eV}$ , this means there are  $N_{\gamma} \approx 1.34 \cdot 10^8$  photons in a pulse. Thus, with a reflection coefficient  $R(1.55\text{eV}) \approx 0.2$ , this means that

$$\eta \approx (1 - R) \frac{N_{\gamma}}{N_{\text{Ru}}} \approx 3.3\text{ppm} \quad (\text{S4})$$

Ru-sites are excited for  $P = 1 \mu\text{W}$  pump power. Alternatively, this corresponds to a photoexcited density of:

$$n_{\gamma} \approx (1 - R) \frac{N_{\gamma}}{V_{\text{u.c.}}} \approx 3.5 \cdot 10^{16} \text{ cm}^{-3} \quad (\text{S5})$$

for the indicated pump power. Each photon will create a hole ( $H$ ) and doublon ( $D$ ) particle, i.e.

$$n_\gamma \equiv n^H = n^D = n_{\text{pair}}^{HD}.$$

## S2 Effective coupling between holon-doublon density and antiferromagnetic order parameter

A microscopical justification of the term  $\propto nL^2$  in the phenomenological free energy  $\mathcal{F}(n, L)$  is given, where  $n$  describes the holon-doublon-pair density and  $L$  the AFM order parameter.

### S2.1 Microscopic Hamiltonian

The starting point of the derivation is a microscopic Hamiltonian describing the spin degrees of freedom and their coupling to the holons-doublons (HD). To this end, we consider the model of Ref. 3, which describes the annihilation of a holon and doublon over a next-nearest neighbor site. The interaction Hamiltonian is given by

$$H_3 = t_3 \sum_{(ijk)ss'} [h_{is} d_{ks'} \vec{\sigma}_{ss'} \cdot \mathbf{S}_j + \text{H.c.}], \quad (\text{S6})$$

where  $h_{is}$  is a fermionic operator annihilating a holon with spin  $s$  on site  $i$ ,  $d_{ks'}$  is a fermionic operator annihilating a doublon with spin  $s'$  on site  $k$ ,  $\vec{\sigma}$  are the Pauli matrices,  $\mathbf{S}_j$  are the effective spin operators on site  $j$ , and  $(ijk)$  denotes indicates that  $i, j, k$  are nearest neighbours (on distinct sites). The next-nearest neighbour hopping amplitude is given by  $t_3$ . We denote the Hamiltonian containing the spins not interacting with the fermions as  $H_0$ .

### S2.2 Perturbative scheme

The free energy can be computed from the partition function  $Z = \text{tr}[e^{-\beta(H_0+H_3)}]$  as  $\mathcal{F} = -\log(Z)/\beta$  (assuming the Boltzmann constant to be unity). Here, we assume that  $H_3$  is a

small perturbation, which should be justified when the HD density is dilute. Accordingly, the partition function can be computed perturbatively as:

$$\frac{Z}{Z_0} = \sum_{n=0}^{\infty} \frac{(-1)^n}{n!} \int_0^\beta d\tau_1 \int_0^\beta d\tau_2 \dots \int_0^\beta d\tau_n \langle T_\tau [H_3(\tau_1) H_3(\tau_2) \dots H_3(\tau_n)] \rangle_0 \quad (\text{S7})$$

where  $Z_0 = \text{tr}[e^{-\beta H_0}]$ ,  $\langle \dots \rangle_0$  denotes thermal average on  $H_0$ , the operators dependence from the imaginary time  $\tau$  is given by  $O(\tau) = e^{\tau H_0} O e^{-\tau H_0}$ , and the symbol  $T_\tau$  denotes imaginary-time ordering, defined as:

$$T_\tau [\Psi(\tau) \Psi^\dagger(\tau')] = \begin{cases} \Psi(\tau) \Psi^\dagger(\tau') & \text{for } \tau > \tau' \\ \pm \Psi(\tau') \Psi^\dagger(\tau) & \text{for } \tau < \tau' \end{cases}, \quad (\text{S8})$$

where the  $\pm$  depends on the field being of bosonic or fermionic nature. Because of the perturbative nature of  $H_3$ , we retain only the leading correction in Eq. (S7). The leading one is the second-order term, since the first-order one vanishes due to  $SU(2)$  symmetry and because it does not conserve the HD number (conserved by  $H_0$ ). In fact:

$$\int_0^\beta d\tau \langle T_\tau [V(\tau)] \rangle_0 = t_3 \sum_{(ijk)ss'} \int_0^\beta d\tau \langle [h_{is}(\tau) d_{ks'}(\tau) \vec{\sigma}_{ss'} \cdot \mathbf{S}_j(\tau) + \text{H.c.}] \rangle_0 = 0. \quad (\text{S9})$$

Notice that the average  $\langle \dots \rangle_0$  factorizes over HD and spin degrees of freedom, as they are decoupled in  $H_0$ . We will therefore focus on the second-order term, which we denote as  $\beta \Delta \mathcal{F}$  for the sake of brevity. In fact, by defining  $\mathcal{F}_0$  the free energy associated with  $Z_0$ , from Eq. (S7) it follows that:

$$\mathcal{F} = -\beta^{-1} \log[Z_0(1 + \beta \Delta \mathcal{F})] \approx \mathcal{F}_0 - \Delta \mathcal{F} \quad (\text{S10})$$

Accordingly, in the following we evaluate  $\Delta \mathcal{F}$ .

### S2.3 Evaluation of $\Delta\mathcal{F}$

The explicit form of  $\Delta\mathcal{F}$  is given by:

$$\begin{aligned}
\Delta\mathcal{F} &= \frac{t_3^2}{\beta} \sum_{\substack{(ijk)ss' \\ (i'j'k')tt'}} \int_{\tau, \tau'} \langle [h_{is}(\tau)d_{ks'}(\tau)\vec{\sigma}_{ss'} \cdot \mathbf{S}_j(\tau) + \text{H.c.}] [h_{i't}(\tau)d_{k't'}(\tau')\vec{\sigma}_{tt'} \cdot \mathbf{S}_{j'}(\tau') + \text{H.c.}] \rangle_0 \\
&= \frac{t_3^2}{\beta} \sum_{\substack{(ijk)ss' \\ (i'j'k')tt'}} \int_{\tau, \tau'} \left[ \langle h_{is}(\tau)d_{ks'}(\tau)d_{k't'}^\dagger(\tau')h_{i't}^\dagger(\tau') \rangle_0 + \langle d_{ks'}^\dagger(\tau)h_{is}^\dagger(\tau)h_{i't}(\tau')d_{k't'}(\tau') \rangle_0 \right] \times \\
&\quad \times \left[ \langle \vec{\sigma}_{ss'} \cdot \mathbf{S}_j(\tau)\vec{\sigma}_{tt'} \cdot \mathbf{S}_{j'}(\tau') \rangle_0 \right], \\
&= \frac{t_3^2}{\beta} \sum_{\substack{(ijk)ss' \\ (i'j'k')}} \int_{\tau, \tau'} \left[ \langle h_{is}(\tau)h_{i's}^\dagger(\tau') \rangle_0 \langle d_{ks'}(\tau)d_{k's'}^\dagger(\tau') \rangle_0 + \langle d_{ks}^\dagger(\tau)d_{k's}(\tau') \rangle_0 \langle h_{is'}^\dagger(\tau)h_{i's'}(\tau') \rangle_0 \right] \times \\
&\quad \times \left[ \langle \mathbf{S}_j(\tau) \cdot \mathbf{S}_{j'}(\tau') \rangle_0 \right],
\end{aligned}$$

with  $\int_{\tau, \tau'} \equiv \int_0^\beta d\tau d\tau'$ , where in the second step we only retain terms conserving the HD number and we factorized the averages, while in the last step we exploit the  $SU(2)$  symmetry. In order to give a coarse-grained version of  $\Delta\mathcal{F}$ , we make the following customary assumptions:

1. we replace  $\langle \mathbf{S}_j(\tau) \cdot \mathbf{S}_{j'}(\tau') \rangle_0 \rightarrow \mathbf{L}_i \cdot \mathbf{L}_j$ , where is a classical AFM order parameter. Other terms in  $\mathbf{L}_j$  can be derived from it, but we only retain the more relevant.
2. We assume all the fields to not depend on  $\tau$ . Further dependences on  $\tau$  are less relevant.
3. We retain only the spatially local part, by neglecting the nearest neighbours contributions, which are less relevant.

The result can then be written as:

$$\begin{aligned}
\Delta\mathcal{F} &= (t_3)^2\beta \sum_i \left[ \sum_{s,s'} \langle h_{is} h_{is}^\dagger \rangle_0 \langle d_{is'} d_{is'}^\dagger \rangle_0 + \sum_{s,s'} \langle d_{is}^\dagger d_{is} \rangle_0 \langle h_{is'}^\dagger h_{is'} \rangle_0 \right] \mathbf{L}_i^2 \\
&= (t_3)^2\beta \sum_i \left[ (2 - n_i^H)(2 - n_i^D) + n_i^H n_i^D \right] \mathbf{L}_i^2 \\
&= (t_3)^2\beta \sum_i \left[ (2 - n_i)^2 + n_i^2 \right] \mathbf{L}_i^2 \\
&\approx (t_3)^2\beta \sum_i \left[ 4 - 4n_i \right] \mathbf{L}_i^2
\end{aligned}$$

where in the second step we defined  $n_i^D = \sum_s \langle h_{is}^\dagger h_{is} \rangle_0$  and  $n_i^H = \sum_s \langle d_{is}^\dagger d_{is} \rangle_0$ , in the third step we used the fact that  $n_i^D = n_i^H \equiv n_i$  (same number of holons and doublons), while in the fourth step we used the diluteness assumption. We end up with a constant term, which simply renormalizes the existing value of the  $\mathbf{L}_i^2$  in  $\mathcal{F}_0$ , and a term coupling the HD density and the square of the order parameter, as desired:

$$\mathcal{F} = \mathcal{F}_0 + 4(t_3)^2\beta \sum_i n_i \mathbf{L}_i^2 \quad (\text{S11})$$

### S3 Nonequilibrium Ginzburg-Landau model

Below, the details of the free energy model are given. The free energy  $\mathcal{F}(n, L)$  has the form:

$$\mathcal{F}(n, L) = \frac{a_1}{2}(n - n_{\text{c,eq}})L^2 + \frac{a_2}{4}L^4 + \tilde{\mathcal{F}}(n), \quad (\text{S12})$$

with

$$\tilde{\mathcal{F}}(n) = a_3 n + \frac{a_4}{2}n^2 + \frac{a_5}{3}n^3 \quad (\text{S13})$$

as discussed in the main text. The equations of motion (eq. 5 in the main manuscript) give the time-evolution of the  $(n, L)$ -coordinates. For a finite cubic term in  $\tilde{\mathcal{F}}(n)$ , i.e.  $a_5 \neq 0$ , the best agreement between model and data is obtained. Forcing the cubic term to be zero ( $a_5 = 0$ )

overestimates the lifetime of the  $L = 0$  plateau, but still shows a good agreement between data and model for the disordering dynamics. Below the model parameters for both cases are shown, in addition to plots of the  $n(t)$ ,  $L(t)$ -coordinates.

### S3.1 $a_5 \neq 0$ , as in the main manuscript

**Table S2:** Model parameters for  $a_5 \neq 0$

| parameter  | value |
|------------|-------|
| $n_{c,eq}$ | 2.165 |
| $a_1$      | 0.92  |
| $a_2$      | 4.95  |
| $a_3$      | -0.21 |
| $a_4$      | 0.27  |
| $a_5$      | 0.06  |

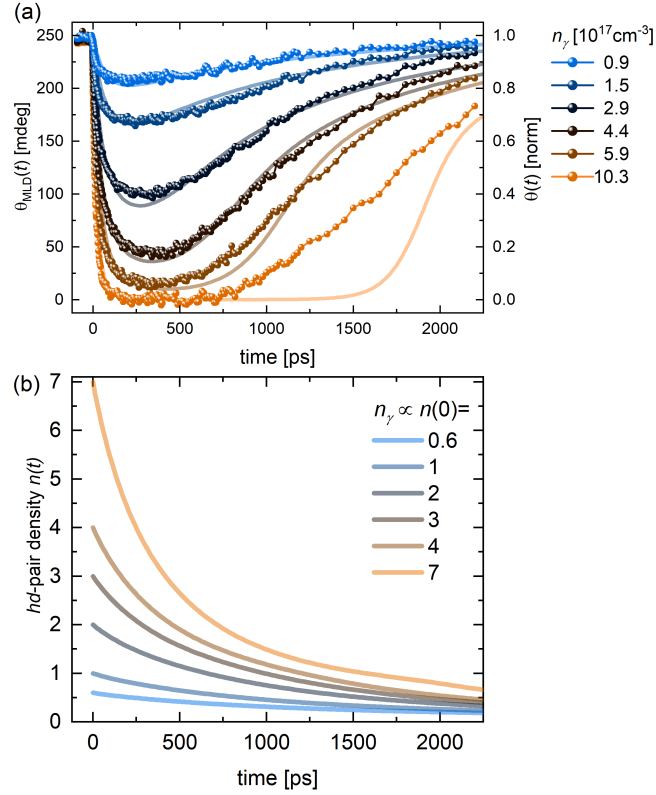

**Figure S2:** a) Data (spheres) and the modelled magnetic linear dichroism induced polarization rotation  $\theta_{MLD}$  for the model with  $a_5 \neq 0$ . b) The  $hd$ -pair density  $n(t)$  curves for different quench strengths.

### S3.2 $a_5 = 0$

**Table S3:** Model parameters for  $a_5 = 0$

| parameter  | value |
|------------|-------|
| $n_{c,eq}$ | 2.33  |
| $a_1$      | 0.94  |
| $a_2$      | 1.675 |
| $a_3$      | -0.63 |
| $a_4$      | 0.52  |
| $a_5$      | 0     |

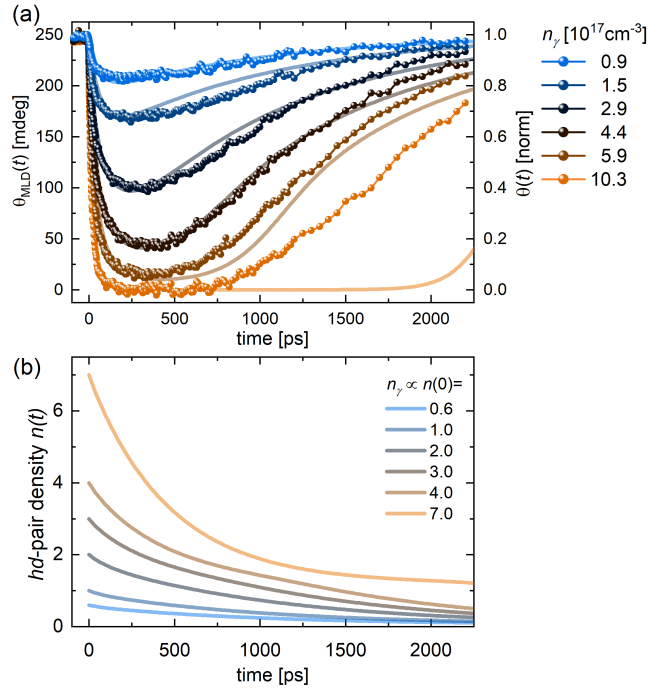

**Figure S3:** a) Data (spheres) and the modelled magnetic linear dichroism induced polarization rotation  $\theta_{MLD}$  for the model with  $a_5 = 0$ . b) The  $hd$ -pair density  $n(t)$  curves for different quench strengths.

## References

1. L. J. Sandilands, C. H. Sohn, H. J. Park, S. Yeun Kim, K. W. Kim, J. A. Sears, Y.-J. Kim, T. Won Noh, Optical probe of Heisenberg-Kitaev magnetism in  $\alpha$ - $\text{RuCl}_3$ , *Phys. Rev. B* **94**, 195156 (2016).
2. R. D. Johnson, S. C. Williams, A. A. Haghighirad, J. Singleton, V. Zapf, P. Manuel, I. I. Mazin, Y. Li, H. O. Jeschke, R. Valentí, R. Coldea, Monoclinic crystal structure of  $\alpha$  -  $\text{RuCl}_3$  and the zigzag antiferromagnetic ground state, *Phys. Rev. B* **92**, 235119 (2015).
3. Z. Lenarčič, P. Prelovšek, Ultrafast charge recombination in a photoexcited Mott-Hubbard insulator, *Phys. Rev. Lett.* **111**, 016401 (2013).
